# Supplementary material for: C-Disentanglement: Discovering Causally-Independent Generative Factors under an Inductive Bias of Confounder
Source: arXiv:2310.17325 source file (2023-10-26)
Supplement: Supplementary file 2 [file app_rebuttal_tables.tex]

\clearpage

\section{Additional Results for Rebuttal}

\textbf{To Reviewer Mytf}

\input{tex/tables/rebuttals/added_UC}

\textbf{To Reviewer TdLu and Reviewer Mytf}

\input{tex/tables/rebuttals/random_label_celebA}




\textbf{To Reviewer j8n4}

\input{tex/tables/rebuttals/added_baselines}


\textbf{Reference}:

[1]Rombach, Robin, et al. "High-resolution image synthesis with latent diffusion models." Proceedings of the IEEE/CVF conference on computer vision and pattern recognition. 2022.

[2]Jeon, Insu, et al. "Ib-gan: Disentangled representation learning with information bottleneck generative adversarial networks." Proceedings of the AAAI Conference on Artificial Intelligence. Vol. 35. No. 9. 2021
